# Supplementary material for: Steady states of two-dimensional granular systems are unique, stable, and sometimes satisfy detailed balance
Source: arXiv:2306.10526 source file (2023-07-07)
Supplement: Supplementary file 1 [file DBUniqueStable_SM.pdf]

# On stability, uniqueness, and detailed balance of steady states in dynamics of planar granular systems: supplemental material

(Dated: June 18, 2023)

## UNIQUENESS OF THE DETAILED-BALANCE SOLUTION FOR $\mathcal{C} = 7$

This proof follows the same rationale as the one for $\mathcal{C} = 6$ in the main text. The existence of the detailed balance solution imposes two restrictions on the values of $\theta_{i,j}$: $\theta_{3,3}\theta_{4,4} = \theta_{3,4}\theta_{3,5}$ and $\theta_{3,3}\theta_{4,5} = \theta_{3,5}\theta_{3,6}$. Since the sum over all the possible $\eta_{i,j}$ vanishes at steady state, the equations reduce to

$$\boldsymbol{\eta} = \begin{bmatrix} \eta_{3,3} \\ \eta_{3,4} \\ \eta_{3,5} \\ \eta_{3,6} \\ \eta_{4,4} \\ \eta_{4,5} \end{bmatrix} = \begin{bmatrix} A+B \\ -B \\ -(A+B) \\ -A \\ B \\ A \end{bmatrix} , \tag{1}$$

where $A \equiv \eta_{4,5}$ and $B \equiv \eta_{4,4}$ are constants. Substituting these in the $\eta$ processes, we have

$$\bar{Q}_4 = (p_{3,3}\bar{Q}_3^2 - (A+B))/q_{3,3} \tag{2a}$$
$$\bar{Q}_5 = (p_{3,4}\bar{Q}_3\bar{Q}_4 + B)/q_{3,4} \tag{2b}$$
$$\bar{Q}_6 = (p_{3,5}\bar{Q}_3\bar{Q}_5 + (A+B))/q_{3,5} \tag{2c}$$
$$\bar{Q}_6 = (p_{4,4}\bar{Q}_4^2 - B)/q_{4,4} \tag{2d}$$
$$\bar{Q}_7 = (p_{3,6}\bar{Q}_3\bar{Q}_6 + A)/q_{3,6} \tag{2e}$$
$$\bar{Q}_7 = (p_{4,5}\bar{Q}_4\bar{Q}_5 - A)/q_{4,5} \ . \tag{2f}$$

The question now is whether or not a steady-state solution exists with $A, B \neq 0$.

There are six different possibilities that have to be checked: $A, B > 0$; $A, B < 0$; $A > |B| > 0, B < 0$; $|B| > A > 0, B < 0$; $B > |A| > 0, A < 0$; $|A| > B > 0, A < 0$. By considering these cases individually and remembering that the $q_{i,j}$ and the $\theta_{i,j}$ are non-negative, each case leads to conflicting relations that cannot exist simultaneously.

1. $A, B > 0$
   From eqs. (2a), (2b), (2c), and (2d), respectively, we have: $\bar{Q}_4 < \theta_{3,3}\bar{Q}_3^2$, $\bar{Q}_5 > \theta_{3,4}\bar{Q}_3\bar{Q}_4$, $\bar{Q}_6 > \theta_{3,5}\bar{Q}_3\bar{Q}_5$, and $\bar{Q}_6 < \theta_{4,4}\bar{Q}_4^2$. Combining these inequalities, we get: $\bar{Q}_6 > \theta_{3,4}\theta_{3,5}\bar{Q}_3^2\bar{Q}_4$ and also $\bar{Q}_6 < \theta_{3,3}\theta_{4,4}\bar{Q}_3^2\bar{Q}_4$. However, this is in conflict with the relation $\theta_{3,3}\theta_{4,4} = \theta_{3,4}\theta_{3,5}$.

2. $A, B < 0$
   This case leads to all the inequality signs of the previous case being reversed, which leads to the same conflict.

3. $A > |B| > 0$ and $B < 0$
   As $A + B > 0$, from (2c) $\bar{Q}_6 > \theta_{3,5}\bar{Q}_3\bar{Q}_5$, whilst from (2a) $\bar{Q}_4 < \theta_{3,3}\bar{Q}_3^2$. Combining these results with (2e) and (2f), we obtain

   $$\bar{Q}_7 > \theta_{3,6}\bar{Q}_3\bar{Q}_6 > \theta_{3,5}\theta_{3,6}\bar{Q}_3^2\bar{Q}_5$$
   $$\bar{Q}_7 < \theta_{4,5}\bar{Q}_4\bar{Q}_5 < \theta_{4,5}\theta_{3,3}\bar{Q}_3^2\bar{Q}_5 \ .$$

   This is in conflict with the condition $\theta_{3,3}\theta_{4,5} = \theta_{3,5}\theta_{3,6}$.

4. $|B| > A > 0$ and $B < 0 \Rightarrow A + B < 0$
   From eqs. (2a), (2d), (2b), and (2c) we obtain, respectively, $\bar{Q}_4 > \theta_{3,3}\bar{Q}_3^2$, $\bar{Q}_6 > \theta_{4,4}\bar{Q}_4^2 > \theta_{3,3}\theta_{4,4}\bar{Q}_3^2\bar{Q}_4$, $\bar{Q}_5 < \theta_{3,4}\bar{Q}_3\bar{Q}_4$, and $\bar{Q}_6 < \theta_{3,5}\bar{Q}_3\bar{Q}_5 < \theta_{3,4}\theta_{3,5}\bar{Q}_3^2\bar{Q}_4$, which are conflicting.

5. $B > |A| > 0$ and $A < 0 \Rightarrow A + B > 0$
   From eqs. (2a), (2b), (2c), and (2d) we obtain, respectively, $\bar{Q}_4 < \theta_{3,3}\bar{Q}_3^2$, $\bar{Q}_5 > \theta_{3,4}\bar{Q}_3\bar{Q}_4$, $\bar{Q}_6 > \theta_{3,5}\bar{Q}_3\bar{Q}_5$, and $\bar{Q}_6 < \theta_{3,3}\bar{Q}_4^2$. From these relations we get $\bar{Q}_6 > \theta_{3,4}\theta_{3,5}\bar{Q}_3^2\bar{Q}_4$, as well as $\bar{Q}_6 < \theta_{3,3}\theta_{4,4}\bar{Q}_3^2\bar{Q}_4$. However, these are in conflict with the relation $\theta_{3,3}\theta_{4,4} = \theta_{3,4}\theta_{3,5}$.

6. $|A| > B > 0$ and $A < 0 \Rightarrow A + B < 0$
   As $A + B < 0$, from (2c) and (2a) we have $\bar{Q}_6 < \theta_{3,5}\bar{Q}_3\bar{Q}_5$ and $\bar{Q}_4 > \theta_{3,3}\bar{Q}_3^2$. Using (2e) and (2f), we then have

   $$\bar{Q}_7 < \theta_{3,6}\bar{Q}_3\bar{Q}_6 < \theta_{3,5}\theta_{3,6}\bar{Q}_3^2\bar{Q}_5$$
   $$\bar{Q}_7 > \theta_{4,5}\bar{Q}_4\bar{Q}_5 > \theta_{4,5}\theta_{3,3}\bar{Q}_3^2\bar{Q}_5 \ .$$

   These are in conflict with $\theta_{3,3}\theta_{4,5} = \theta_{3,5}\theta_{3,6}$.

Thus, all the six combinations of $A$ and $B$ do not lead to realisable solutions and the detailed-balance solution is the only possible steady state.

## THE NUMERICAL ANALYSIS FOR $\mathcal{C} = 6$

The goal of the numerical investigation is to explore the solutions to

$$\bar{Q}_4 = (p_{3,3}\bar{Q}_3^2 - A)/q_{3,3}, \tag{3a}$$
$$\bar{Q}_5 = (p_{3,4}\bar{Q}_3\bar{Q}_4 + A)/q_{3,4}, \tag{3b}$$
$$\bar{Q}_6 = (p_{3,5}\bar{Q}_3\bar{Q}_5 + A)/q_{3,5}, \tag{3c}$$
$$\bar{Q}_6 = (p_{4,4}\bar{Q}_4^2 - A)/q_{4,4} \tag{3d}$$

and, in particular, search for sets of parameters that admit multiple solutions.

We applied the *Solve* function in Mathematica to eqs. (3), with the normalisation restriction, $\bar{Q}_3 + \bar{Q}_4 + \bar{Q}_5 +$

| $\bar{Q}_3$ | $\bar{Q}_4$ | $\bar{Q}_5$ | $\bar{Q}_6$ |
|---|---|---|---|
| 0.42 | 0.33 | 0.16 | 0.09 |
| -1 | -1.41 | 4.83 | -1.41 |
| -1 | 1.41 | -0.83 | 1.41 |
| -3.55 | 3.76 | 8.10 | -7.31 |
| -0.18 - 0.55i | -1.55 + 0.13i | 1.37 + 1.10i | 1.36 - 0.68i |
| -0.18 + 0.55i | -1.55 - 0.13i | 1.37 - 1.10i | 1.36 + 0.68i |

TABLE I. The steady-state solutions of (3) with $p_{3,3} = 1$ and $p_{i,j} = 1$ for all other $i, j$ and $q_{i,j} = 1$ for all $i, j$.

| $p_{3,3}$ | $p_{3,4}$ | $p_{3,5}$ | $p_{4,4}$ | $q_{3,3}$ | $q_{3,4}$ | $q_{3,5}$ | $q_{4,4}$ |
|---|---|---|---|---|---|---|---|
| 0.1 | 0.1 | 0.1 | 0.1 | 0.1 | 0.1 | 0.1 | 0.1 |
| 0.1 | 0.1 | 0.1 | 0.1 | 0.1 | 0.1 | 0.1 | 0.5 |
| 0.1 | 0.1 | 0.1 | 0.1 | 0.1 | 0.1 | 0.1 | 1.0 |
| 0.1 | 0.1 | 0.1 | 0.1 | 0.1 | 0.1 | 0.1 | 3.0 |
| 0.1 | 0.1 | 0.1 | 0.1 | 0.1 | 0.1 | 0.5 | 0.1 |

TABLE II. First five combinations of the sampled parameter space.

$\bar{Q}_6 = 1$. An example investigation of the set $p_{3,3} = 2$, all other $p_{i,j} = 1$, and all $q_{i,j} = 1$ is displayed in Table I. There are six solutions in total, of which three have negative $Q$-fractions and another two have complex fractions. Thus, only one of the solutions (the first row) is physical. This example is typical of all the sets of parameters we investigated.

To explore the space of rate parameters, we assigned each rate one of four values: 0.1, 0.5, 1.0, and 3.0, and investigated all the possible $4^8$ case combinations as follows. We first determined the number of *physical* solutions by imposing an additional restriction on *solve*: $0 \leq \bar{Q}_i \leq 1$. Then, we looped over all the possible values of the above rates. The sampling method of the parameter space is illustrated in Table II for the first five, out of the $4^8 = 65536$, cases.

Not finding any parameter combination that yields more than one physical solution in our numerical exploration could be significant. It seems to support our conjecture in the main text that only one physical solution exists, for any set of the rate parameters, $q_{i,j}$ and $p_{i,j}$, even when that solution does not satisfy detailed balance.

## THE NUMERICAL ANALYSIS FOR $\mathcal{C} = 7, 8$

To analyse the equations for $\mathcal{C} = 7$ and $\mathcal{C} = 8$, some slight modifications were made to the code. Firstly the equations which were used in *Solve* were the appropriate ones for systems of these orders. The physicality conditions were imposed and the systems solved in the same manner. The one major difference is the size of the parameter space. In particular for $\mathcal{C} = 7$ there are 12 rates and for $\mathcal{C} = 8$ there are 18 rates. This necessitated a different approach in sampling the parameter space. In particular the rates were allowed to take on either of two values and all possible combinations were analysed. This was performed for six sets in the case of $\mathcal{C} = 7$: $\{0.1, 0.5\}, \{0.1, 1\}, \{0.1, 2\}, \{0.5, 1\}, \{0.5, 2\}, \{1, 2\}$, in total 24576 different systems. For $\mathcal{C} = 8$ it was performed for two sets: $\{0.1, 0.5\}$ and $\{0.5, 2\}$, in total 524288 different systems. The equations rarely yield detailed-balance solutions and an example of a standard, non detailed-balance steady state is shown in Fig. 1.

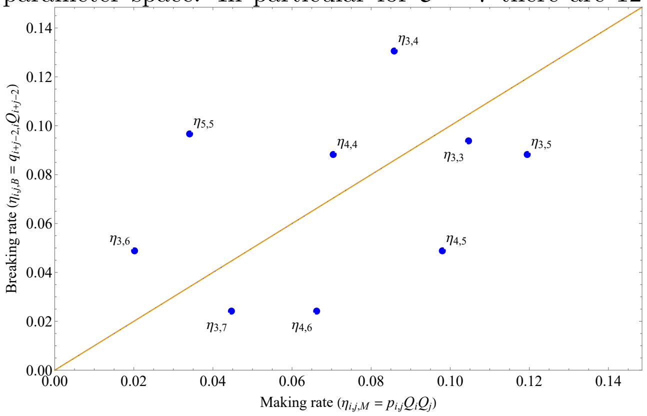


FIG. 1. The unique physical steady state for $\mathcal{C} = 8$, with the parameters $p_{3,3} = p_{3,4} = p_{3,5} = p_{3,7} = p_{4,4} = p_{4,5} = p_{4,6} = 3$, $q_{5,5} = 2$ and all other $p_{i,j}$ and $q_{i,j}$ equal to 0.5. The labels indicate the respective rates. The steady state rates do not lie on the solid line and, therefore, the system does not satisfy detailed-balance.
